# Supplementary material for: Distributed Function Chaining with Anycast Routing
Source: arXiv:1810.03355 source file (2018-10-08)
Supplement: Supplementary file 1 [file appendix.tex]

\appendix
\section{Metric and weight computation}

\textbf{Calcul des métriques. } A chaque cycle le MANO récupère la valeur en pps émise pour chaque VNF. Il utilise cette valeur et l'annonce sur le réseau. 

\textbf{Calcul des poids pour WCMP. } Chaque D-MANO récupère les annonces comportant les métriques pour un type de VNF i donné ainsi que le coût réseau pour l'atteindre. On note le coût réseau $n_{i,k}$ et le coût de la VNF $v_{i,k}$ où i correspond au type de VNF et k à l'instance. On note le coût total $c_{i,k} = n_{i,k} + v_{i,k}$. 

On calcule le poids par la formule: $w_i,k =\frac{1}{1+C_{i,k}}$. On retranscrit ainsi que plus le coût augmente, plus le poids est faible. On note $W_i$ la somme de tous les poids d'instance de vnf sur le réseau pour un type de vnf donnée ($W_i = \sum_{k} w_{i,k}$). Pour obtenir une probabilité entre 0 et 1 on normalise ensuite le poids. On a donc $p_{i,k} = \frac{w_{i,k}}{W_i}$
